# Supplementary material for: Variance reduction with practical all-to-all lattice propagators
Source: arXiv:1402.0831 source file (2016-07-07)
Supplement: Supplementary file 1 [file appendix.tex]

\appendix
\section{Trace over quark loops}\label{app:plots}
\begin{figure*}
\centering
%\vspace{-2.0cm}
\subfigure{
  \includegraphics[scale=0.22]{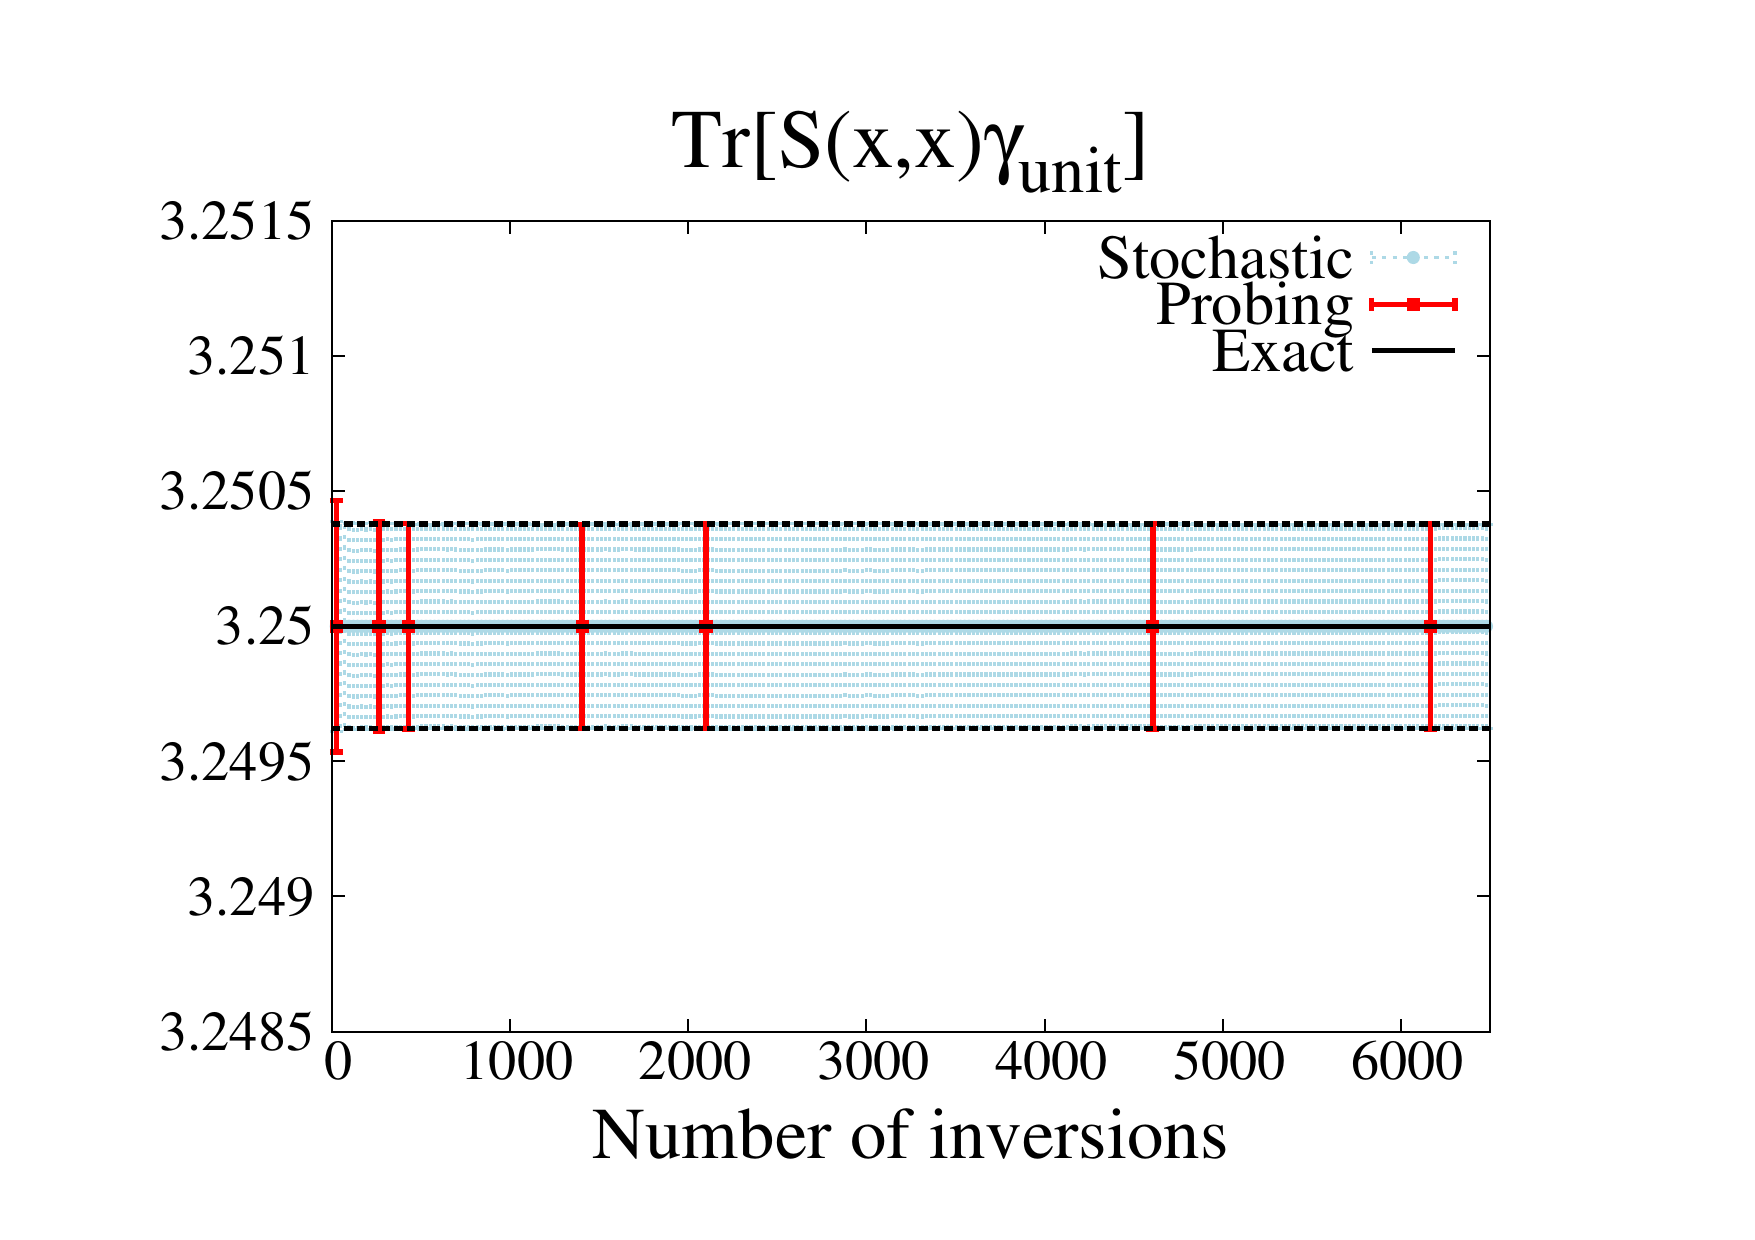}
    \label{fig:app:collect_unit_8}
}
\hspace{1.0cm}
\subfigure{
  \includegraphics[scale=0.22]{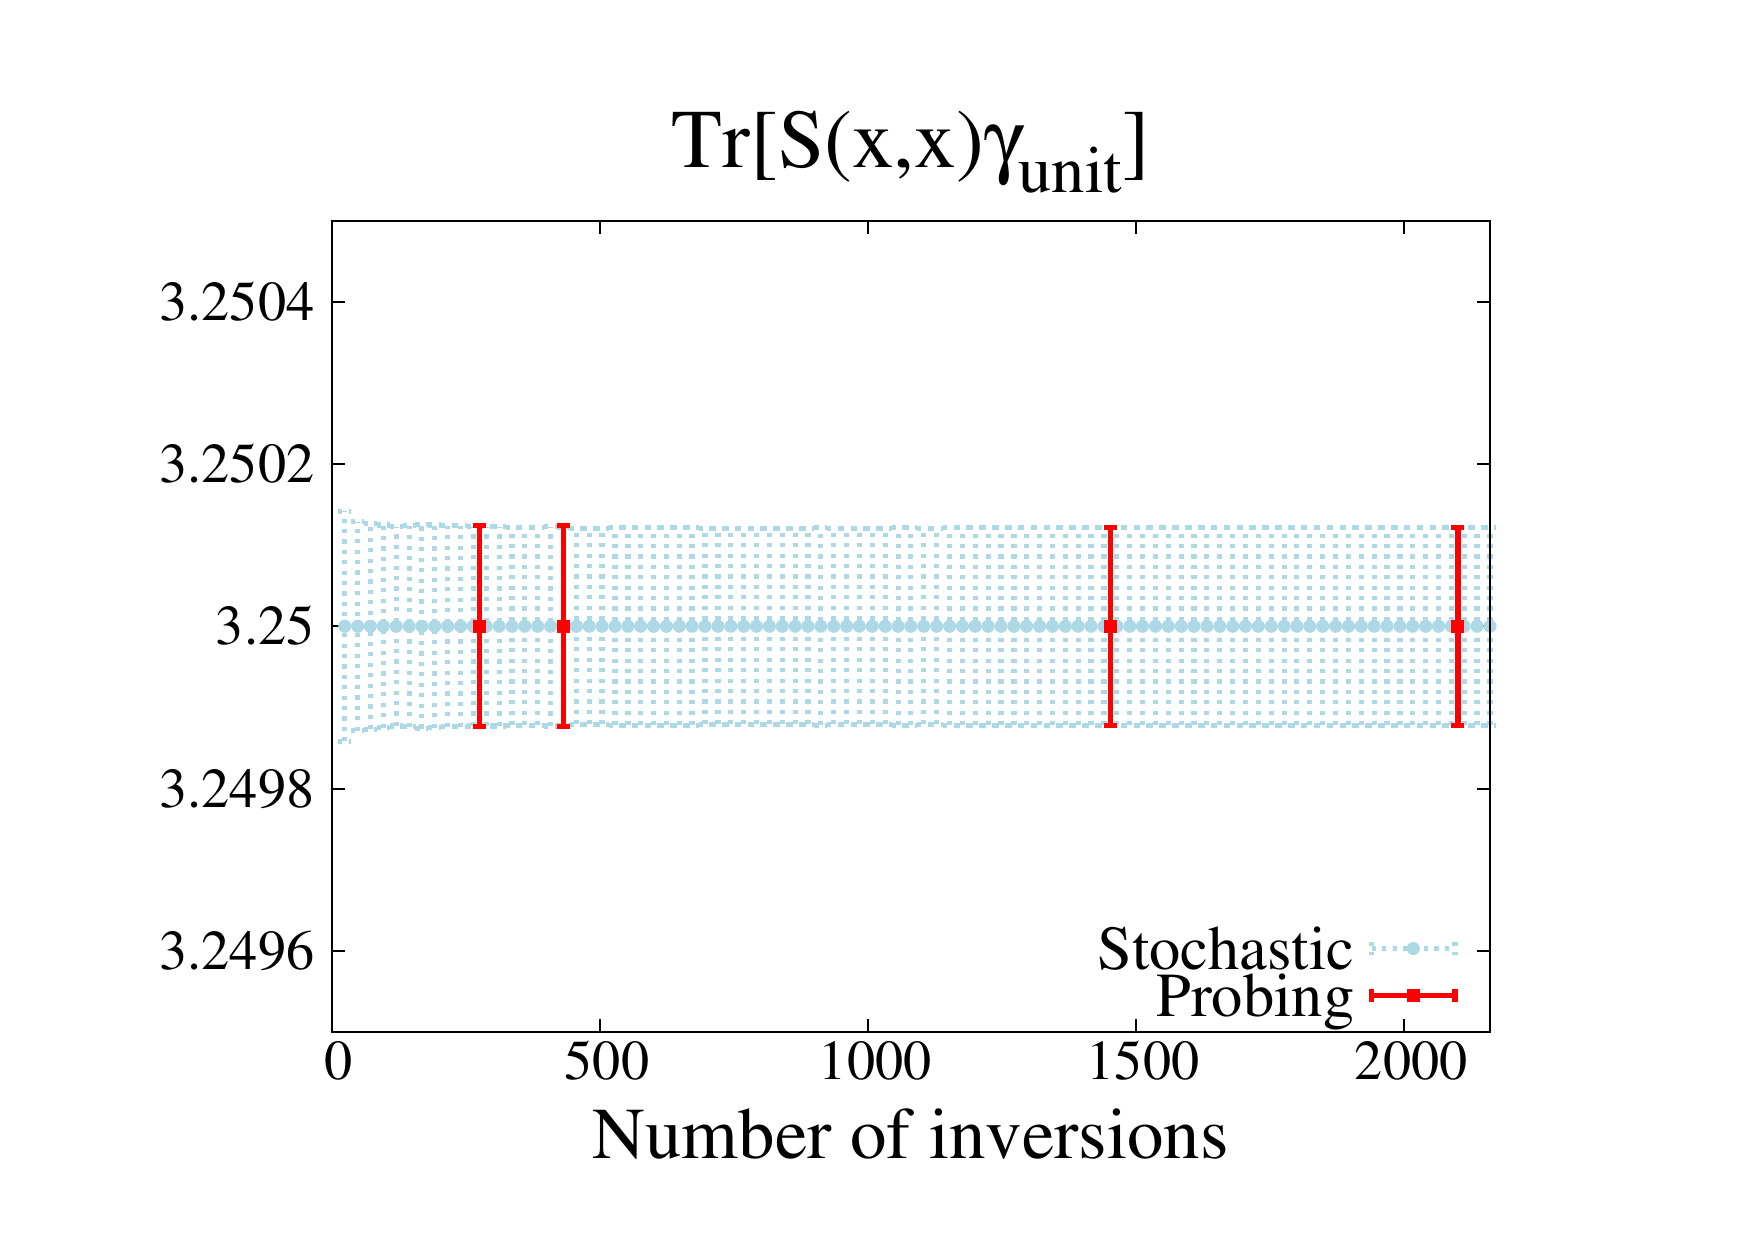}
    \label{fig:app:collect_unit_16}
}\\
\vspace{-0.5cm}
\subfigure{
  \includegraphics[scale=0.22]{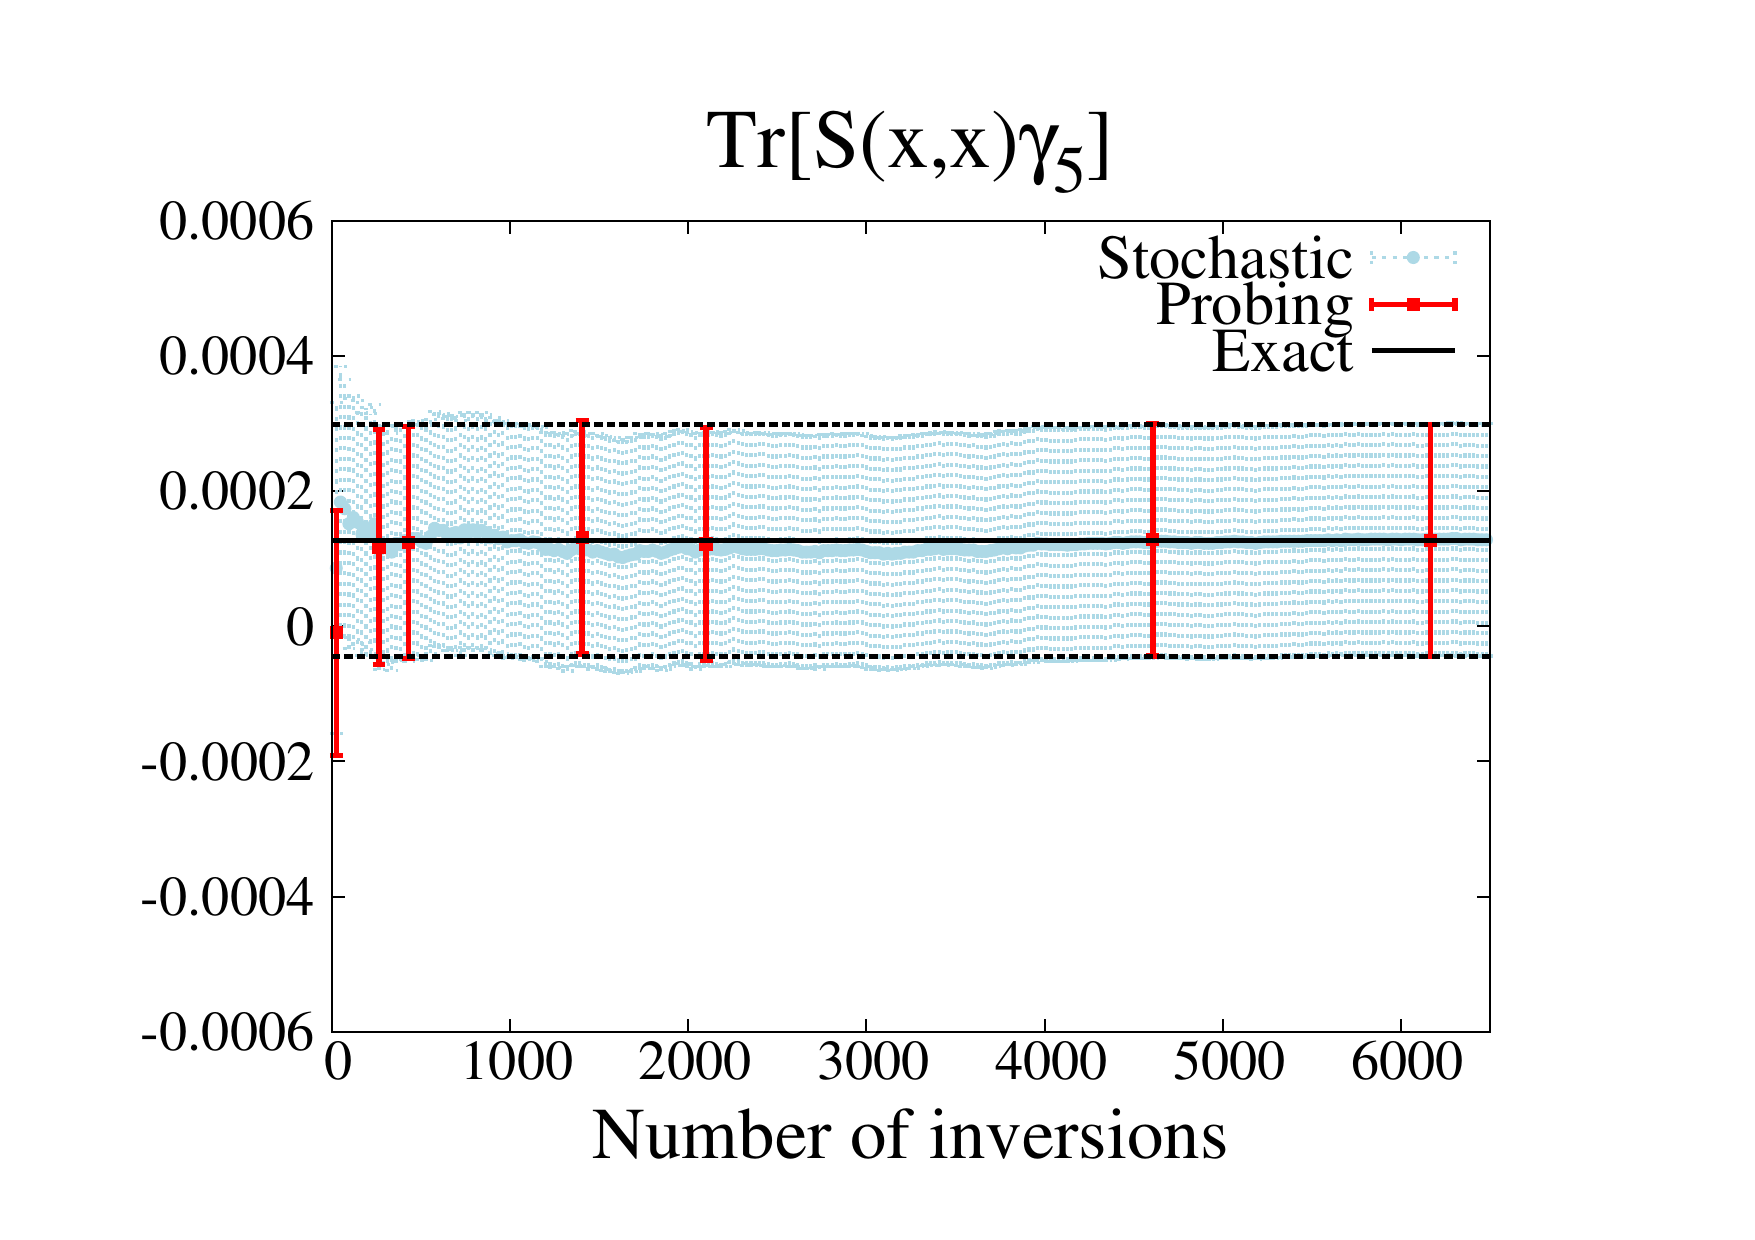}
    \label{fig:app:collect_5_8}
}
\hspace{1.0cm}
\subfigure{
  \includegraphics[scale=0.22]{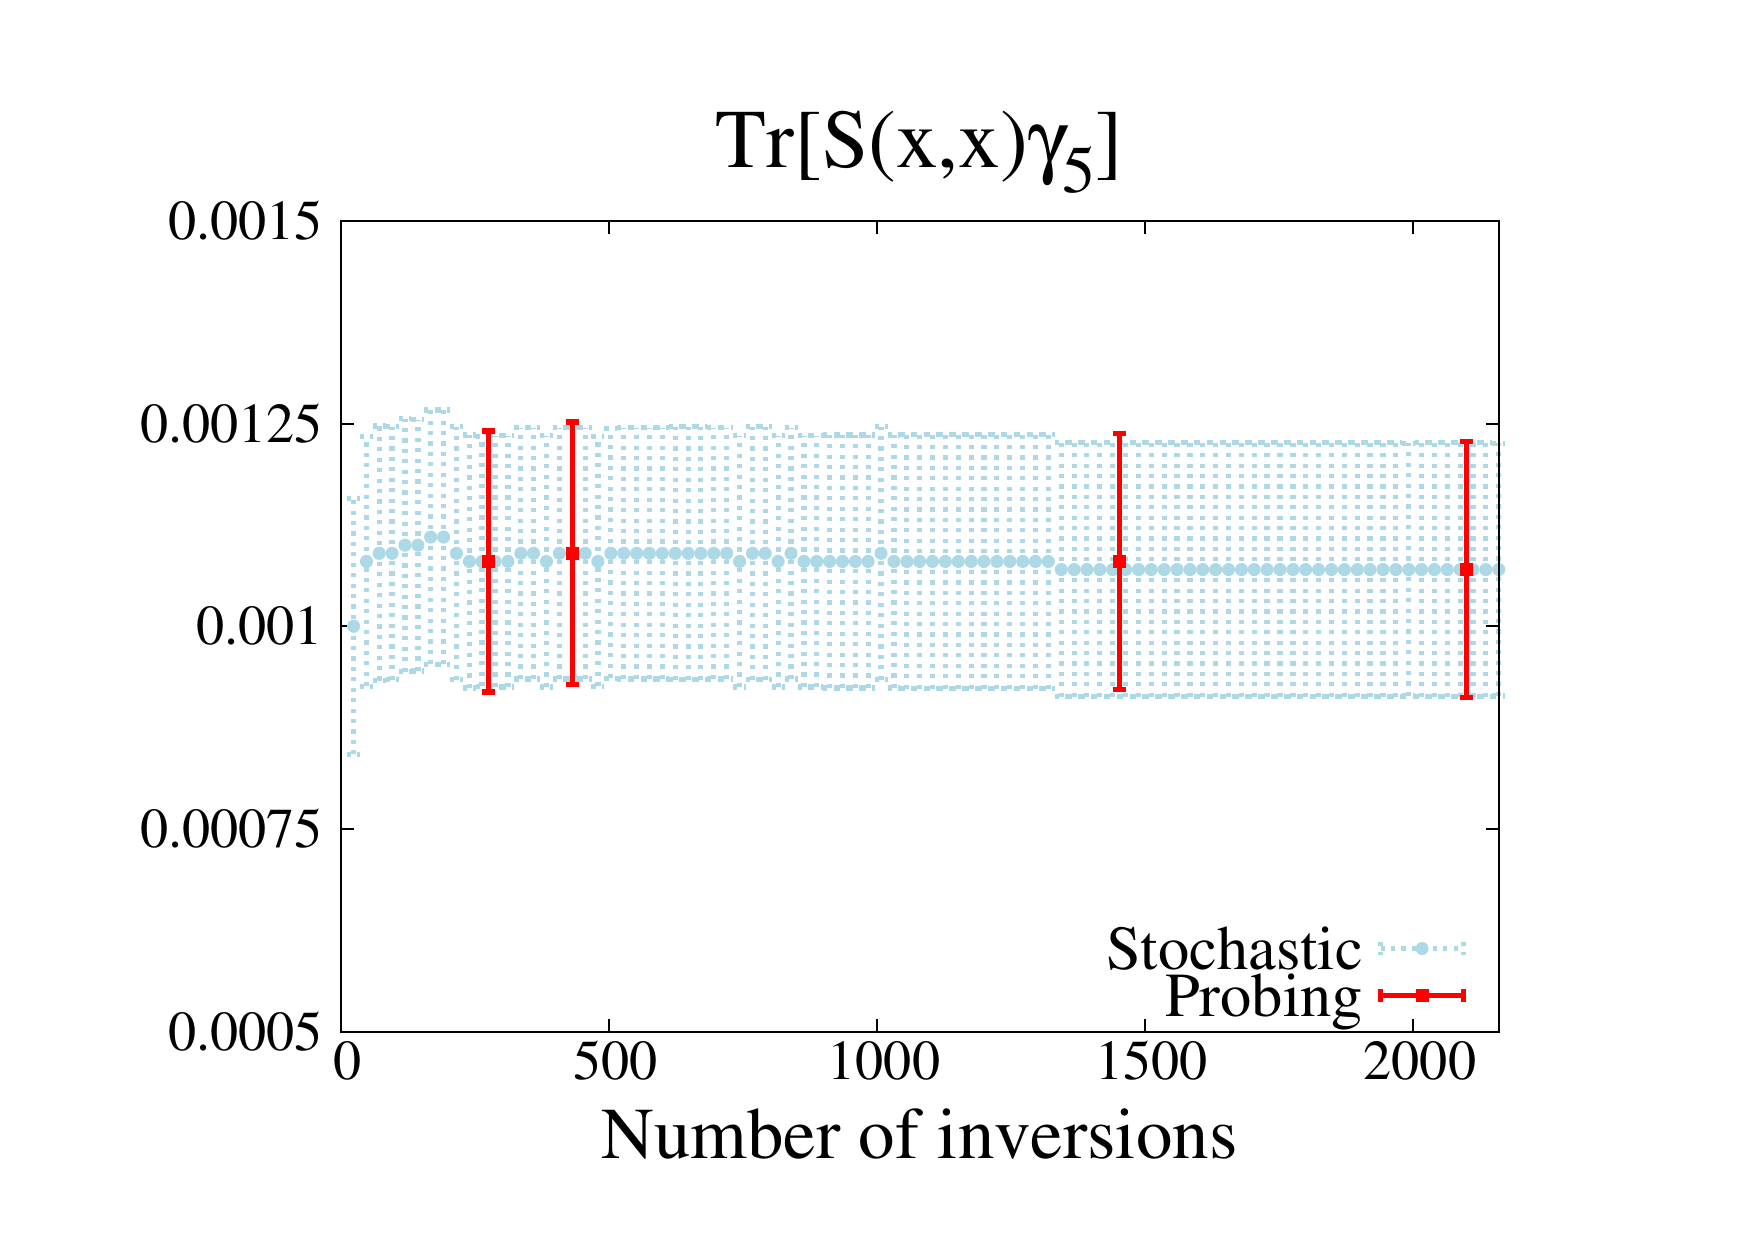}
    \label{fig:app:collect_5_16}
}\\
\vspace{-0.5cm}
\subfigure{
  \includegraphics[scale=0.22]{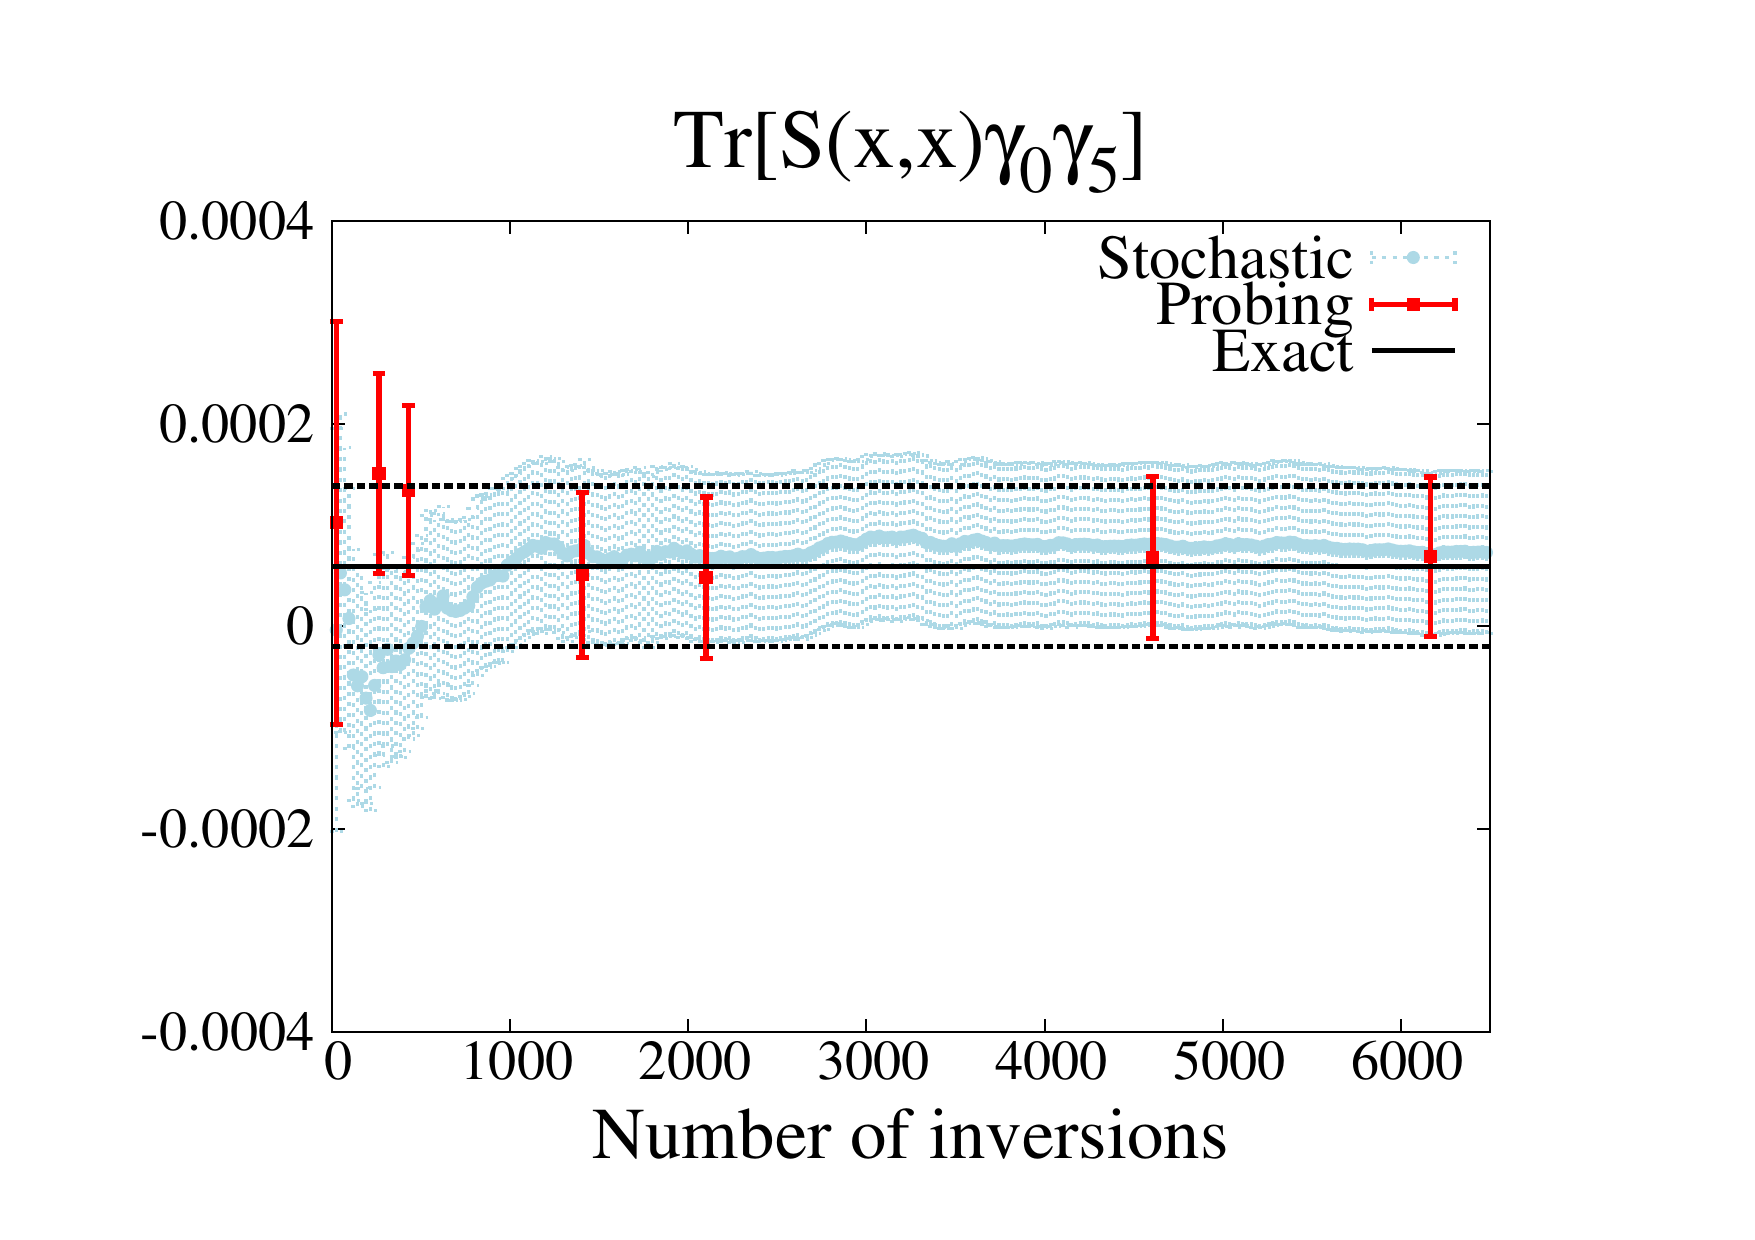}
    \label{fig:app:collect_05_8}
}
\hspace{1.0cm}
\subfigure{
  \includegraphics[scale=0.22]{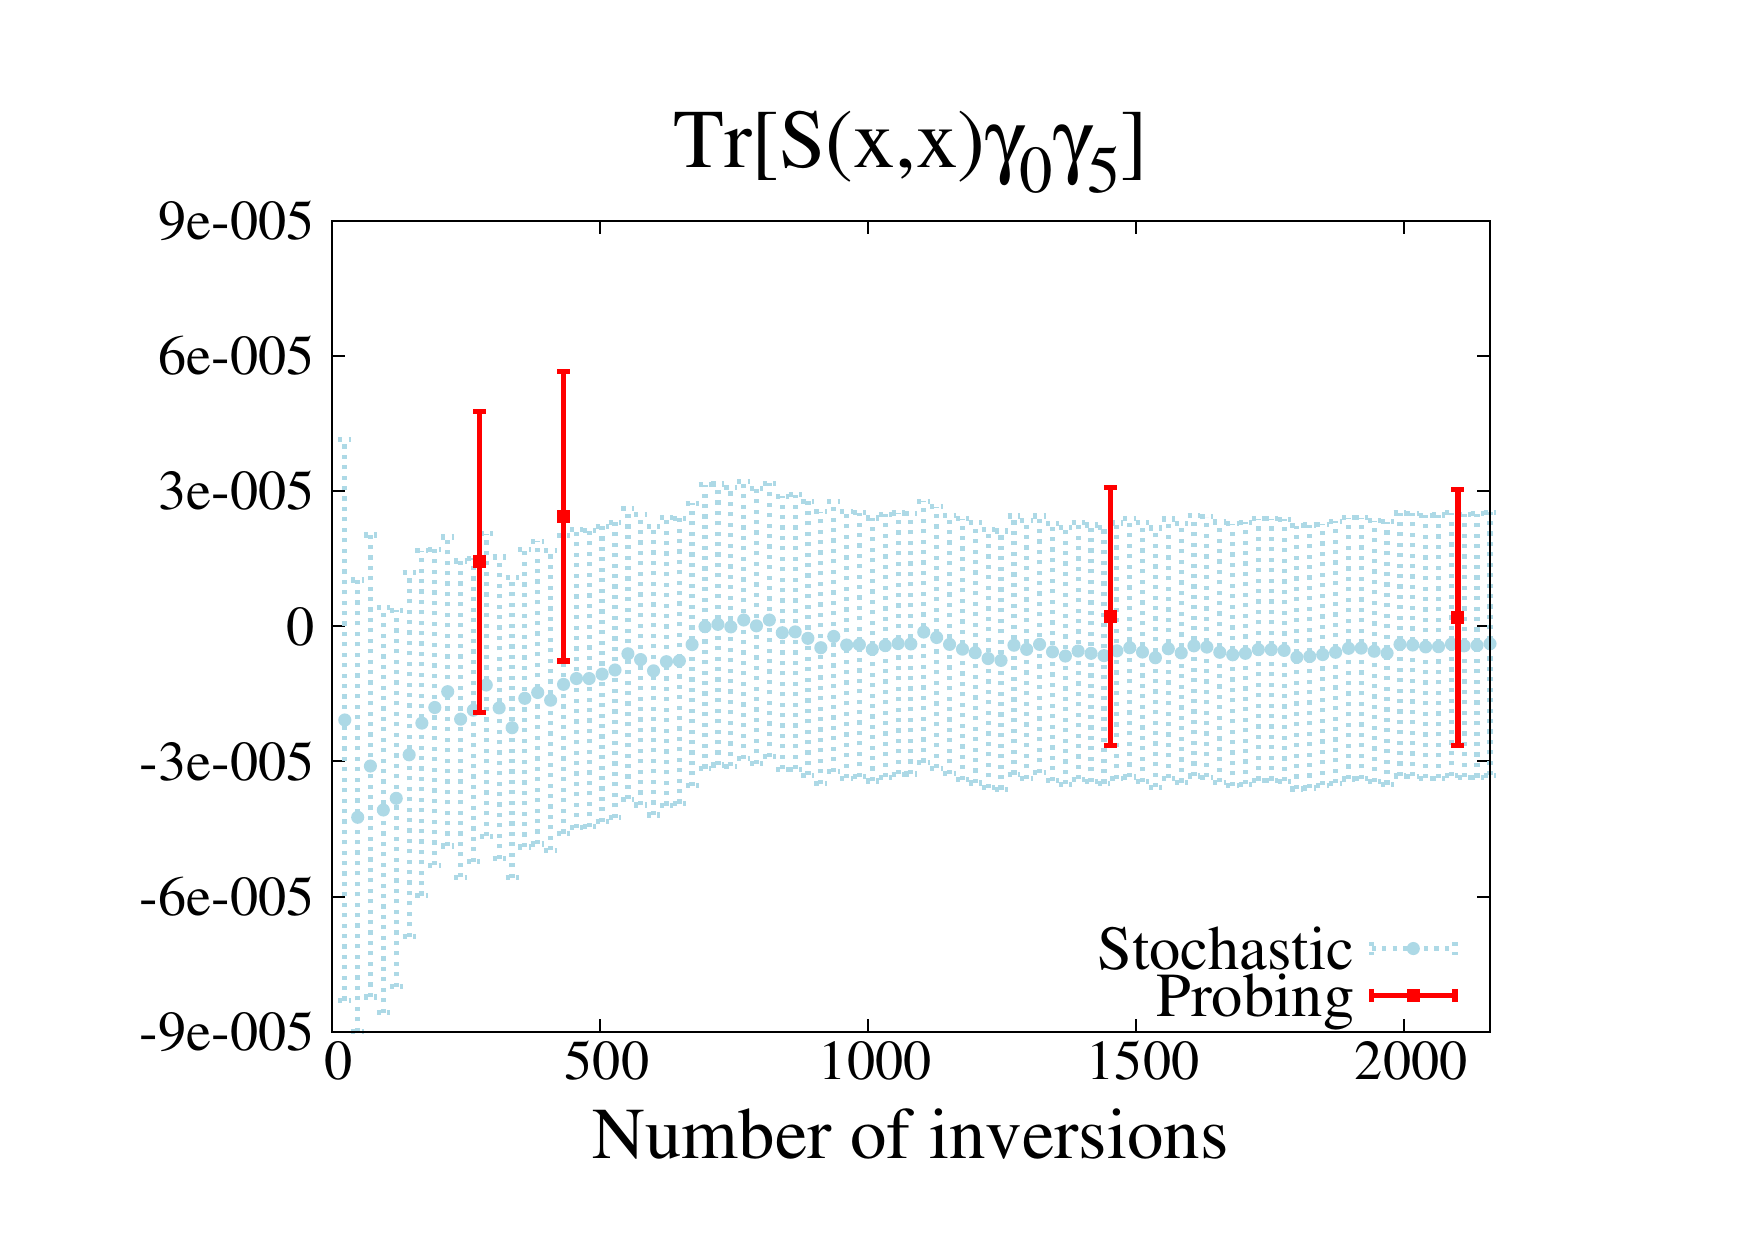}
    \label{fig:app:collect_05_16}
}\\
\vspace{-0.5cm}
\subfigure[Volume $8^{4}$]{
  \includegraphics[scale=0.22]{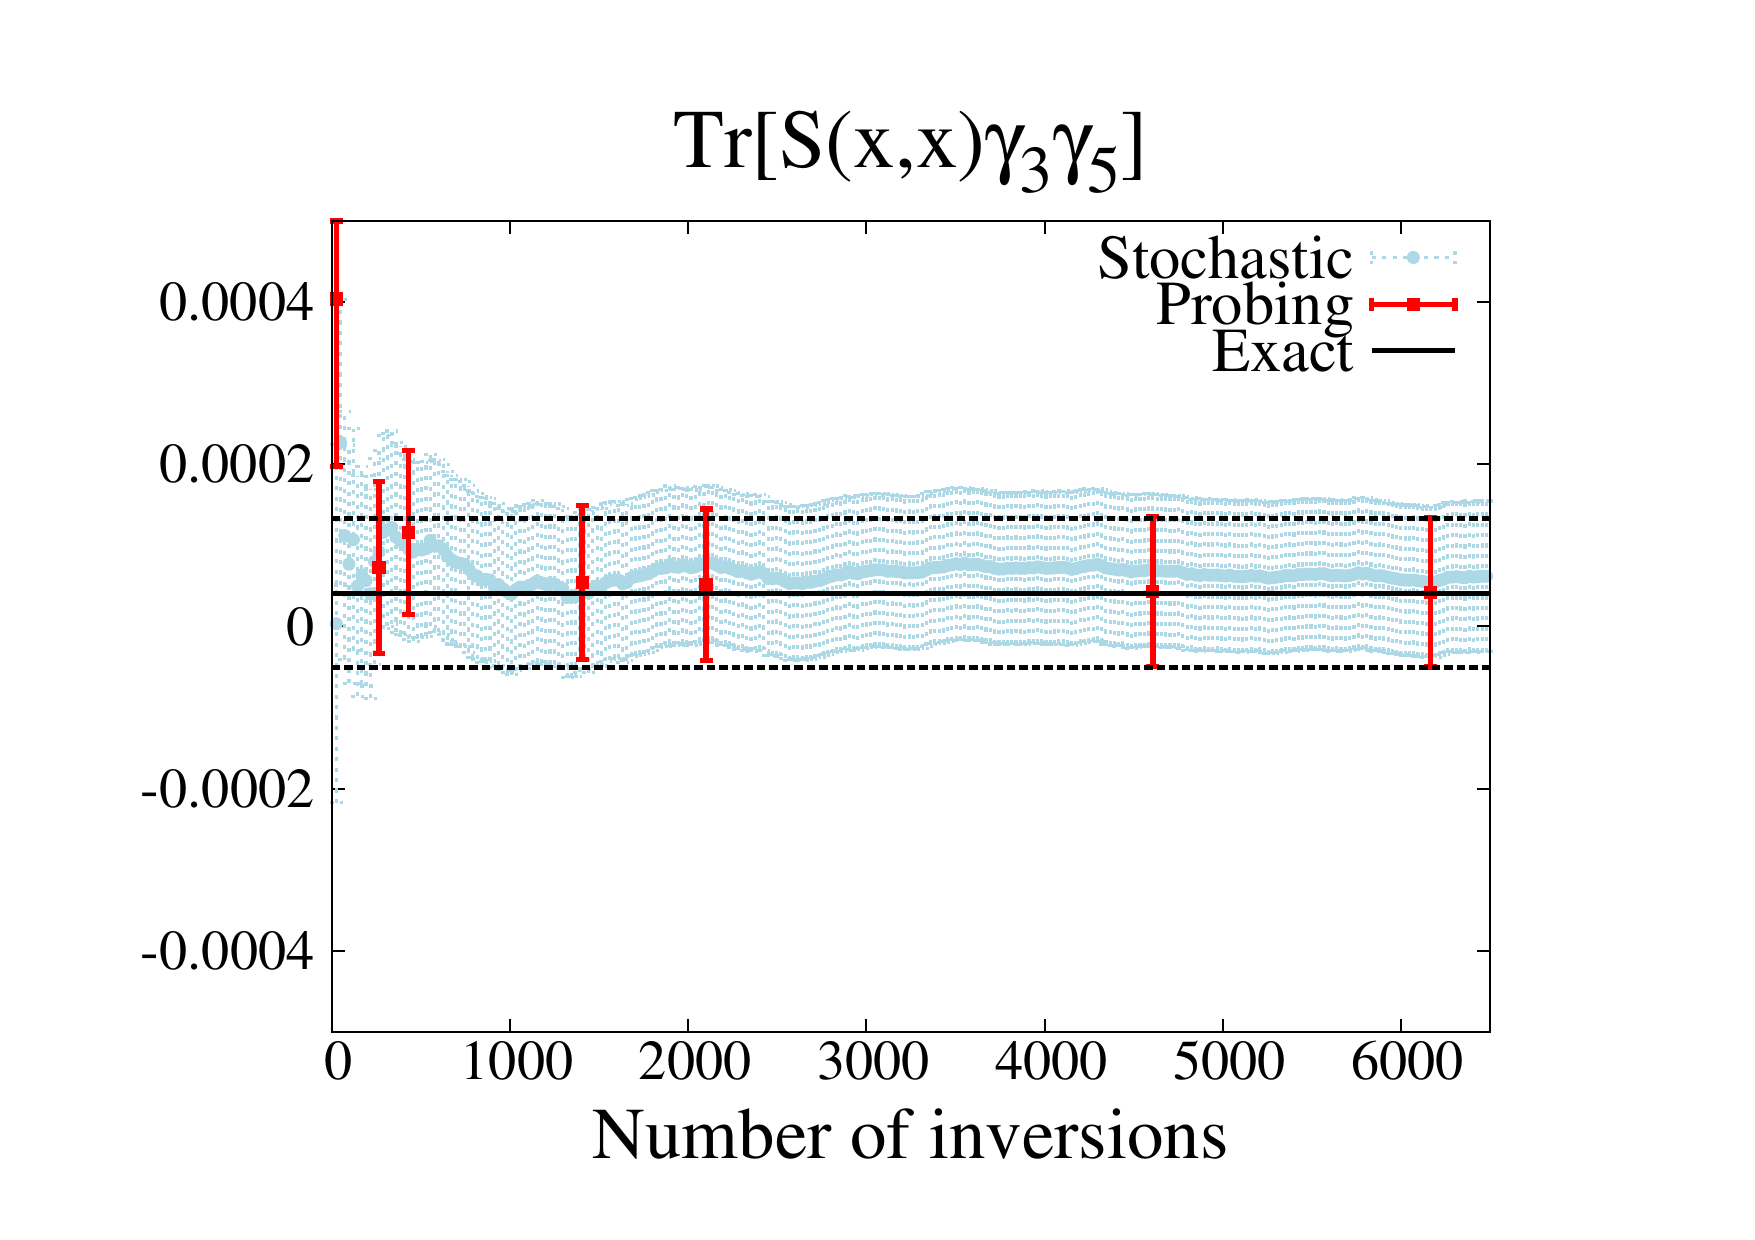}
    \label{fig:app:collect_35_8}
}
\hspace{1.0cm}
\subfigure[Volume $16^{4}$]{
  \includegraphics[scale=0.22]{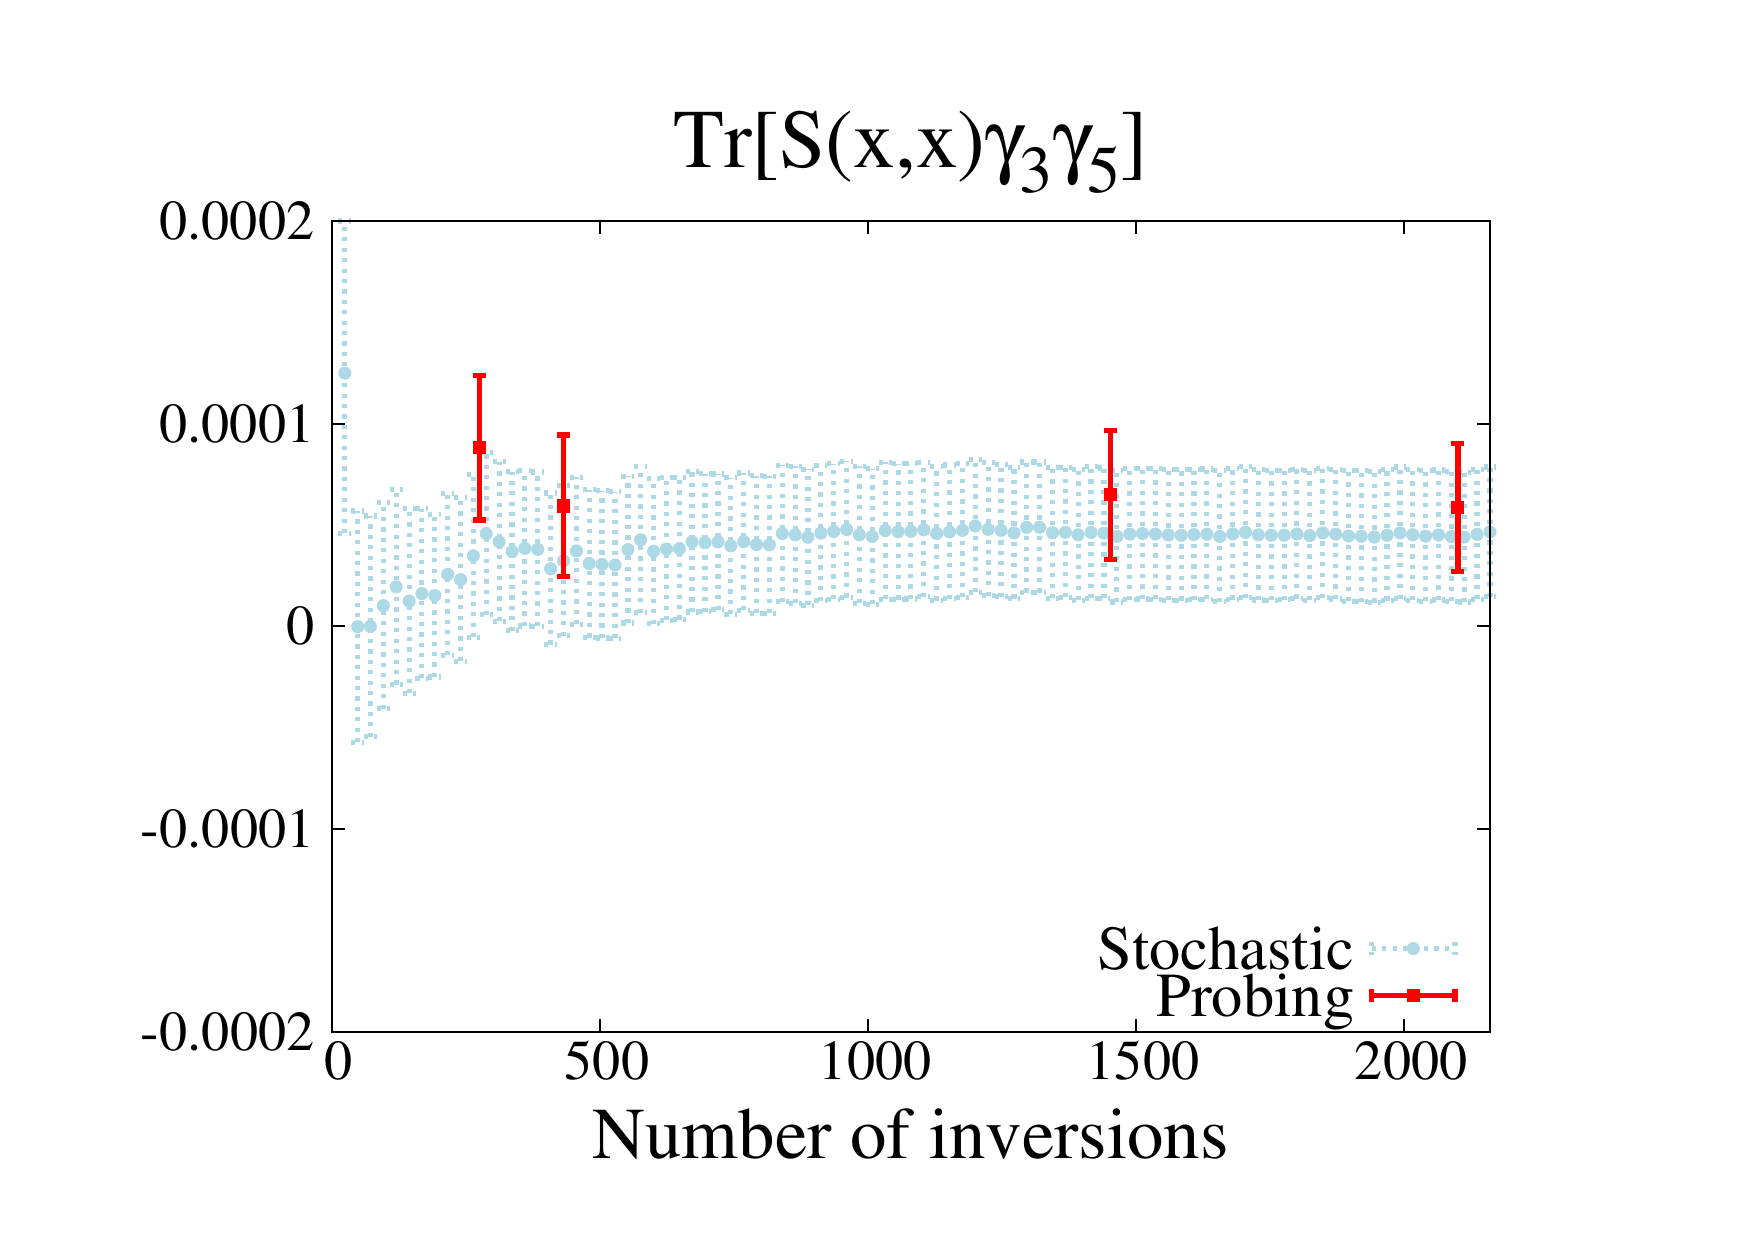}
    \label{fig:app:collect_35_16}
}
\caption[Optional caption for list of figures]{Trace over a closed loop propagator with the insertion of $\Gamma=\gamma_{3}^{}\gamma_{5}^{}$. Red (solid) bars correspond to the probing method for $p=1,\dots,7$ (smaller volume) and $p=2,\dots,5$ (larger volume). The results of the stochastic technique are denoted by blue (dashed) bars. For the smaller volume the exact solution is illustrated by the black (solid) line with its range of error constrained by the black (dashed) lines}
\label{fig:app:collect_IV}
\end{figure*}
